# Supplementary material for: Layout-induced Video Representation for Recognizing Agent-in-Place Actions
Source: arXiv:1804.01429 source file (2019-04-01)
Supplement: Supplementary file 1 [file supp.tex]

% \section{Supplementary Materials}

% \section{Action Dataset Comparison}
% We compare the property of 

\begin{figure*}[!t]
\centering
  \includegraphics[width=0.6\linewidth]{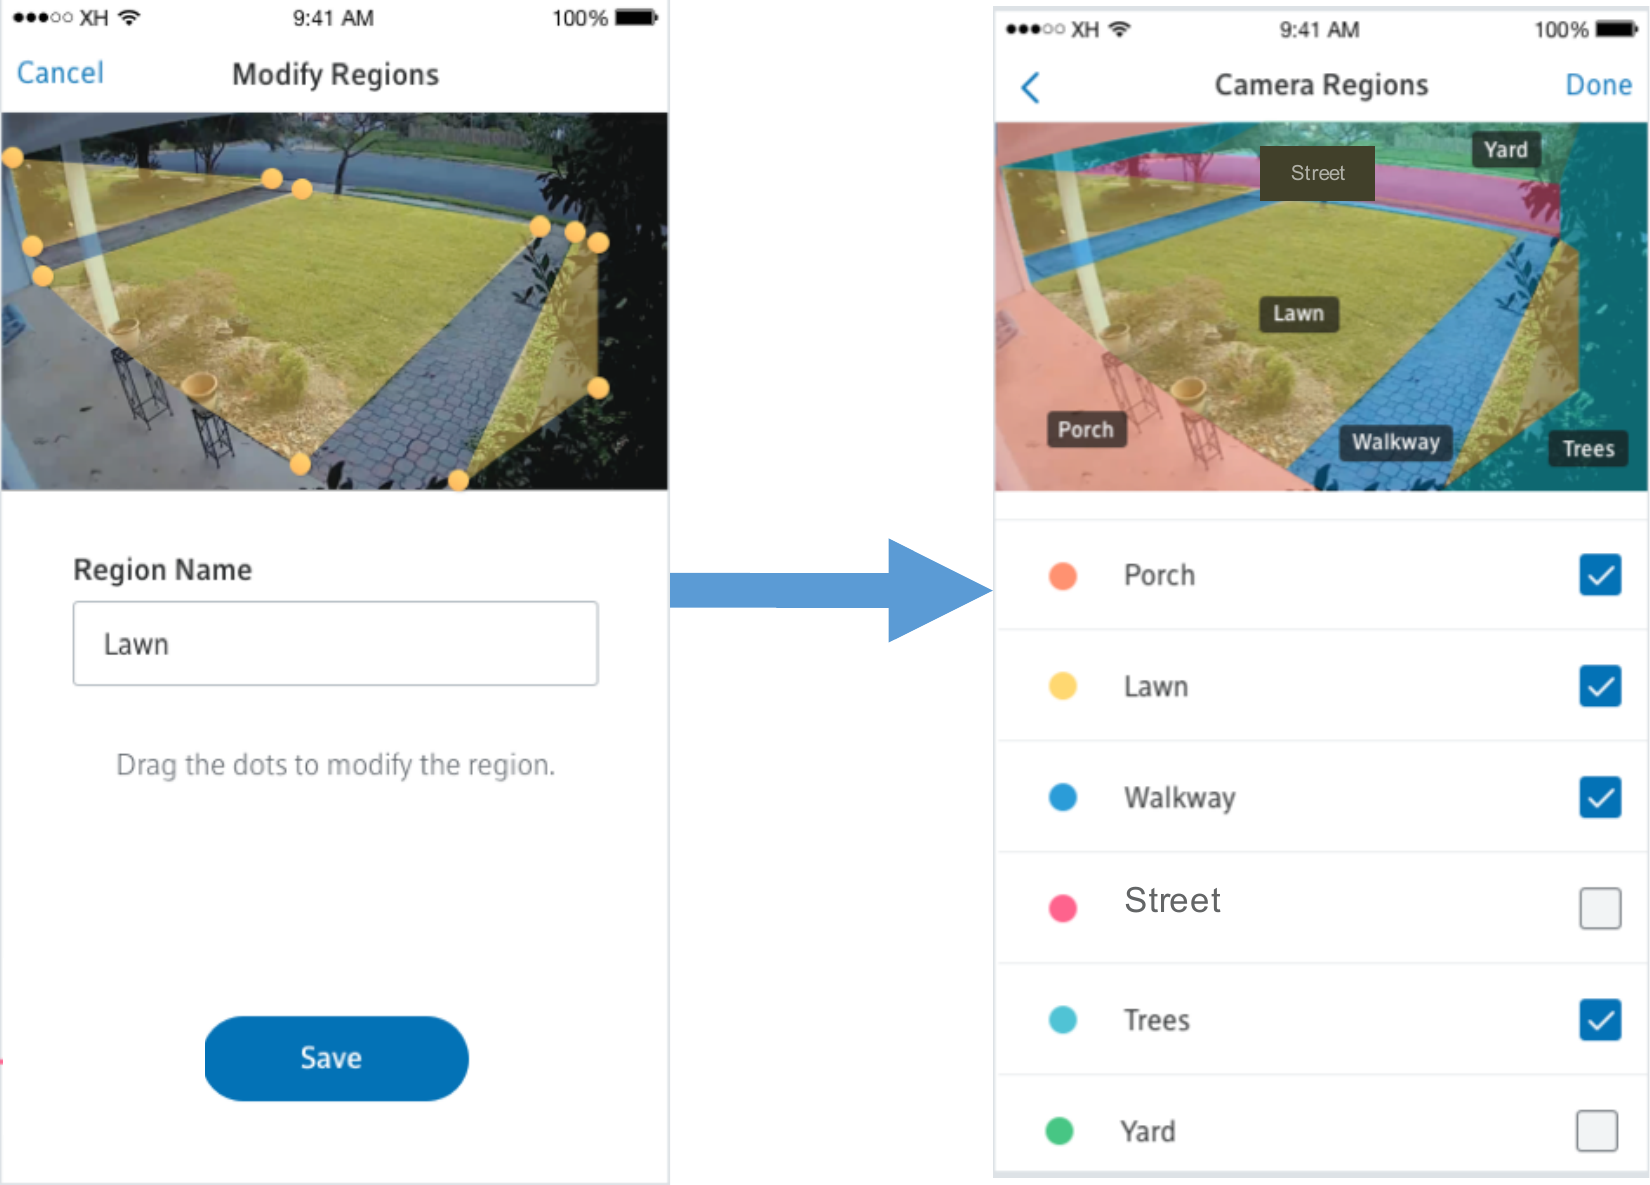}
  \caption{Mobile app for users to annotate camera regions. Note that this version of App contains not only the six places in the main paper but also some more fine-grained places.}
\label{fig:ST_pool}
\end{figure*}

\section{Mobile App for Annotating Places}
We developed a mobile app for users to efficiently annotate their camera regions. The app is shown in Figure \ref{fig:ST_pool}. Users can simply use points to define polygons and choose a pre-defined category for each place. The annotation process is efficient since usually the users will fix the cameras for a long time, and they only need to spend a few seconds to annotate the segmentation maps one time per camera.

\section{Dataset Statistics}
Detailed dataset statistics are shown in Table \ref{data}.

\begin{table*}[!h]
\centering
\scriptsize
\caption{Dataset Statistics}
\label{data}
\begin{tabular}{c|cc|c}
\toprule
                                           & Observed Scene & Unseen Scene & Total \\
                                           \midrule
<vehicle, move along, street>                & 1397	&957	&2354
  \\
<person,move along,sidewalk>               & 539	&299	&838
   \\
<pet,move along,sidewalk>                  & 149	&169	&318
   \\
<person,stay,lawn>                      & 54	&129	&183
   \\
<person,move away (home),driveway>      & 218	&173	&391
   \\
<person,move toward (home),driveway>    & 222	&201	&423
   \\
<person,move toward (home),walkway>     & 153	&91	&244
   \\
<person,move away (home),walkway>       & 118	&52	&170
   \\
<vehicle,move away (home),driveway>     & 71	&70	&141
  \\
<vehicle,move toward (home),driveway>   & 52	&66	&118
   \\
<person,interact with vehicle,driveway> & 171	&81	&252
   \\
<person,move across,lawn>               & 225	&433	&658
   \\
<person,stay,porch>                     & 105	&112	&217
   \\
<person,move toward (home),porch>       & 310	&139	&449
  \\
<person,move away (home),porch>         & 260	&136	&396
   \\
\midrule
Total                                      & 4044	&3108	&7152

\\ \bottomrule
\end{tabular}
\end{table*}

\section{Network Architecture}
The architecture of our network is shown in Table \ref{network}.
\begin{table*}[!h]
\centering
\scriptsize
\caption{Network Structure of LIVR. We apply spatial-only max pooling after block Conv1-Conv5, and temporal-only max pooling after block Conv6-Conv9. From Conv3 to Conv9, each conv blocks consists of two identical 3D-conv layers with ReLU in between. The "on/off" status of each connection for the final gated FC layer is determined by Topo-Agg.}
\label{network}
\begin{tabular}{@{}c|c|c|c|c|c|c|c|c|c|c@{}}
\toprule
Block     & Input Size  & Kernel Size & Stride & \begin{tabular}[c]{@{}c@{}}\# Filters\end{tabular} &            & Block     & Input Size  & Kernel Size & Stride & \begin{tabular}[c]{@{}c@{}}\# Filters\end{tabular}\\ \midrule
Conv1     & 15$\times$90$\times$160$\times$3 & 3$\times$3$\times$3       & 1$\times$1$\times$1  & 64 & &Conv6     & 15$\times$3$\times$5$\times$64   & 3$\times$3$\times$3       & 1$\times$1$\times$1  & 64    \\
Pool1     & 15$\times$90$\times$160$\times$3 & 1$\times$2$\times$2       & 1$\times$2$\times$2  & -  & &Pool6     & 15$\times$3$\times$5$\times$64   & 2$\times$1$\times$1       & 2$\times$1$\times$1  & -    \\
Conv2     & 15$\times$45$\times$80$\times$64 & 3$\times$3$\times$3       & 1$\times$1$\times$1  & 64  &   &Conv7     & 8$\times$3$\times$5$\times$64    & 3$\times$3$\times$3       & 1$\times$1$\times$1  & 64 \\
Pool2     & 15$\times$45$\times$80$\times$64 & 1$\times$2$\times$2       & 1$\times$2$\times$2  & -   & &Pool7     & 8$\times$3$\times$5$\times$64    & 2$\times$1$\times$1       & 2$\times$1$\times$1  & -    \\
Conv3     & 15$\times$23$\times$40$\times$64 & 3$\times$3$\times$3       & 1$\times$1$\times$1  & 64  &  & Conv8     & 4$\times$3$\times$5$\times$64    & 3$\times$3$\times$3       & 1$\times$1$\times$1  & 64  \\
Pool3     & 15$\times$23$\times$40$\times$64 & 1$\times$2$\times$2       & 1$\times$2$\times$2  & -   &  &Pool8     & 4$\times$3$\times$5$\times$64    & 2$\times$1$\times$1       & 2$\times$1$\times$1  & -   \\
Conv4     & 15$\times$12$\times$20$\times$64 & 3$\times$3$\times$3       & 1$\times$1$\times$1  & 64  &  &Conv9     & 2$\times$3$\times$5$\times$64    & 3$\times$3$\times$3       & 1$\times$1$\times$1  & 64   \\
Pool4     & 15$\times$12$\times$20$\times$64 & 1$\times$2$\times$2       & 1$\times$2$\times$2  & -   & &Pool9     & 2$\times$3$\times$5$\times$64    & 2$\times$1$\times$1       & 2$\times$1$\times$1  & -    \\
Conv5     & 15$\times$6$\times$10$\times$64  & 3$\times$3$\times$3       & 1$\times$1$\times$1  & 64  & &SGMP       & 1$\times$3$\times$5$\times$64    & 1$\times$3$\times$5       & 1$\times$1$\times$1  & -       \\
Pool5     & 15$\times$6$\times$10$\times$64  & 1$\times$2$\times$2       & 1$\times$2$\times$2  & -  & & Gated FC & 1$\times$1$\times$1$\times$384    & -          &  -       & -       \\ \bottomrule
\end{tabular}
\end{table*}

\section{Decoupling Spatial-temporal Max Pooling}
Traditional 3D ConvNets conduct max pooling along both spatial and temporal dimensions of feature maps to increase the size of receptive field. In home surveillance scenario, it is reported in \cite{remotenet} that decoupling the max pooling by first conducting spatial-only max pooling on some 3D-conv blocks, then adding more conv blocks with temporal-only max pooling leads to better performance. One possible reason is that conducting temporal-wise max pooling early will capture motion patterns of only local body of the moving objects. Since in a home surveillance video, the moving objects are usually large, and we need to apply several conv blocks with spatial-only max pooling layers to capture the motion of the entire object.
We tried both methods and the per-category average precision results is shown in Fig.\ref{fig:ST_pool}. "ST Max Pool" denotes that we use 5 conv blocks with spatial-temporal max pooling to abstract both spatial and temporal information at the same time. "Decouple ST Max Pool" denotes our network structure that has 5 conv blocks with spatial-only max pooling, and followed by 4 more blocks with temporal-only max pooling. Since the second network has more conv blocks, to make the two network structures have similar depth, we add one more conv layer in each conv block of "ST Max Pool". For both methods, we use our full model with PD+DD+Topo-Agg. The hyper-parameters setting is: we decompose semantics on different places after the second conv blocks ($L=2$); we conduct distance-based place discretization on $PL_{DT} = \{\emph{\text{walkway}}, \emph{\text{driveway}}, \emph{\text{lawn}}\}$ and choose $k=3$; for topological feature aggregation, we choose $h=1$. We can observe that "Decouple ST Max Pool" leads to better performance.

\begin{figure*}[!h]
\centering
  \includegraphics[width=0.9\linewidth]{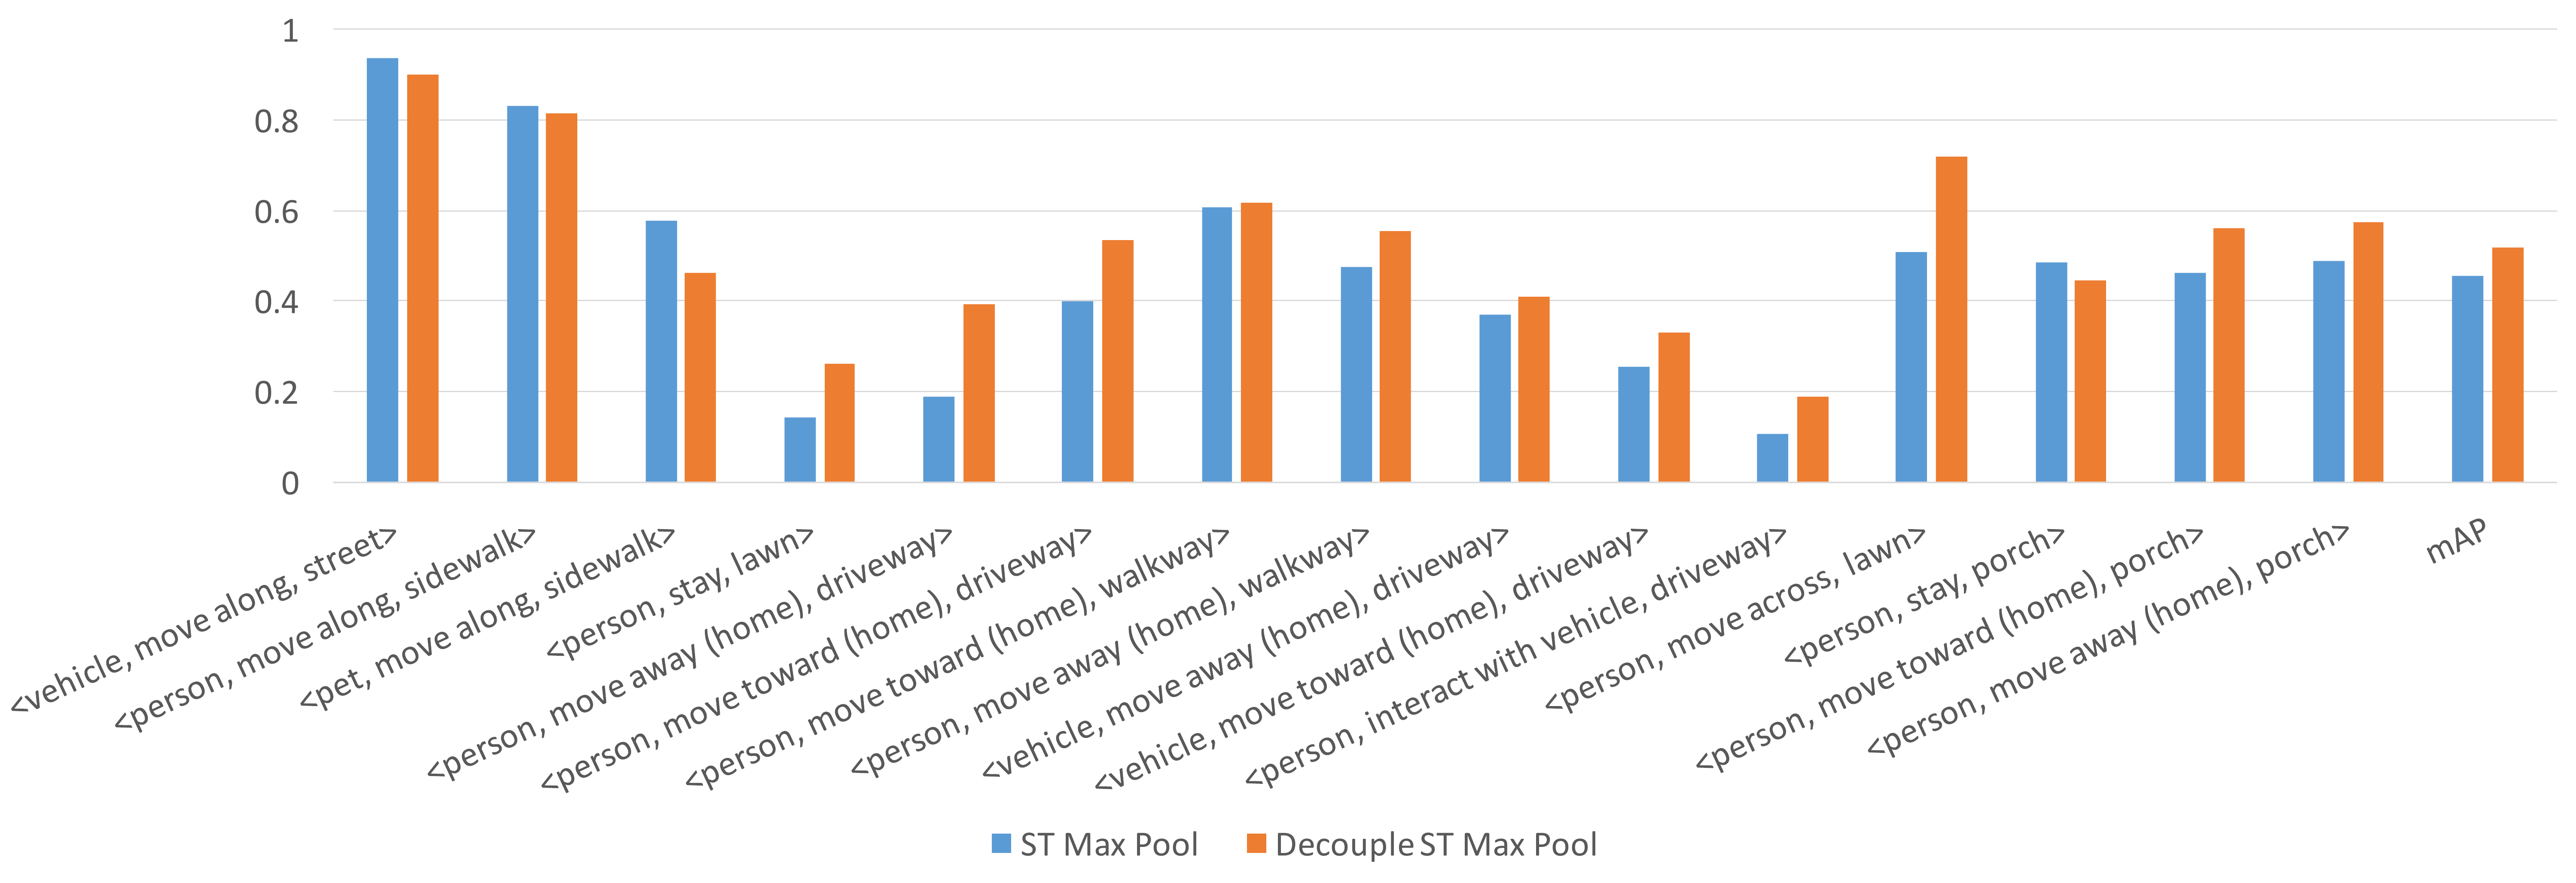}
  \caption{"ST Max Pool" denotes a network structure with 5 conv blocks with spatial-temporal max pooling. "Decouple ST Max Pool" denotes our network structure that has 5 conv blocks with spatial-only max pooling, and followed by 4 more blocks with temporal-only max pooling. We observe performance improvements on almost all action categories.}
\label{fig:ST_pool}
\end{figure*}

% \section{Baseline Models}
% The network structures of the baseline models are shown in Fig.\ref{fig:BL12} and \ref{fig:BL3}.
% \begin{figure}[!t]
% \centering
%   \includegraphics[width=0.8\linewidth]{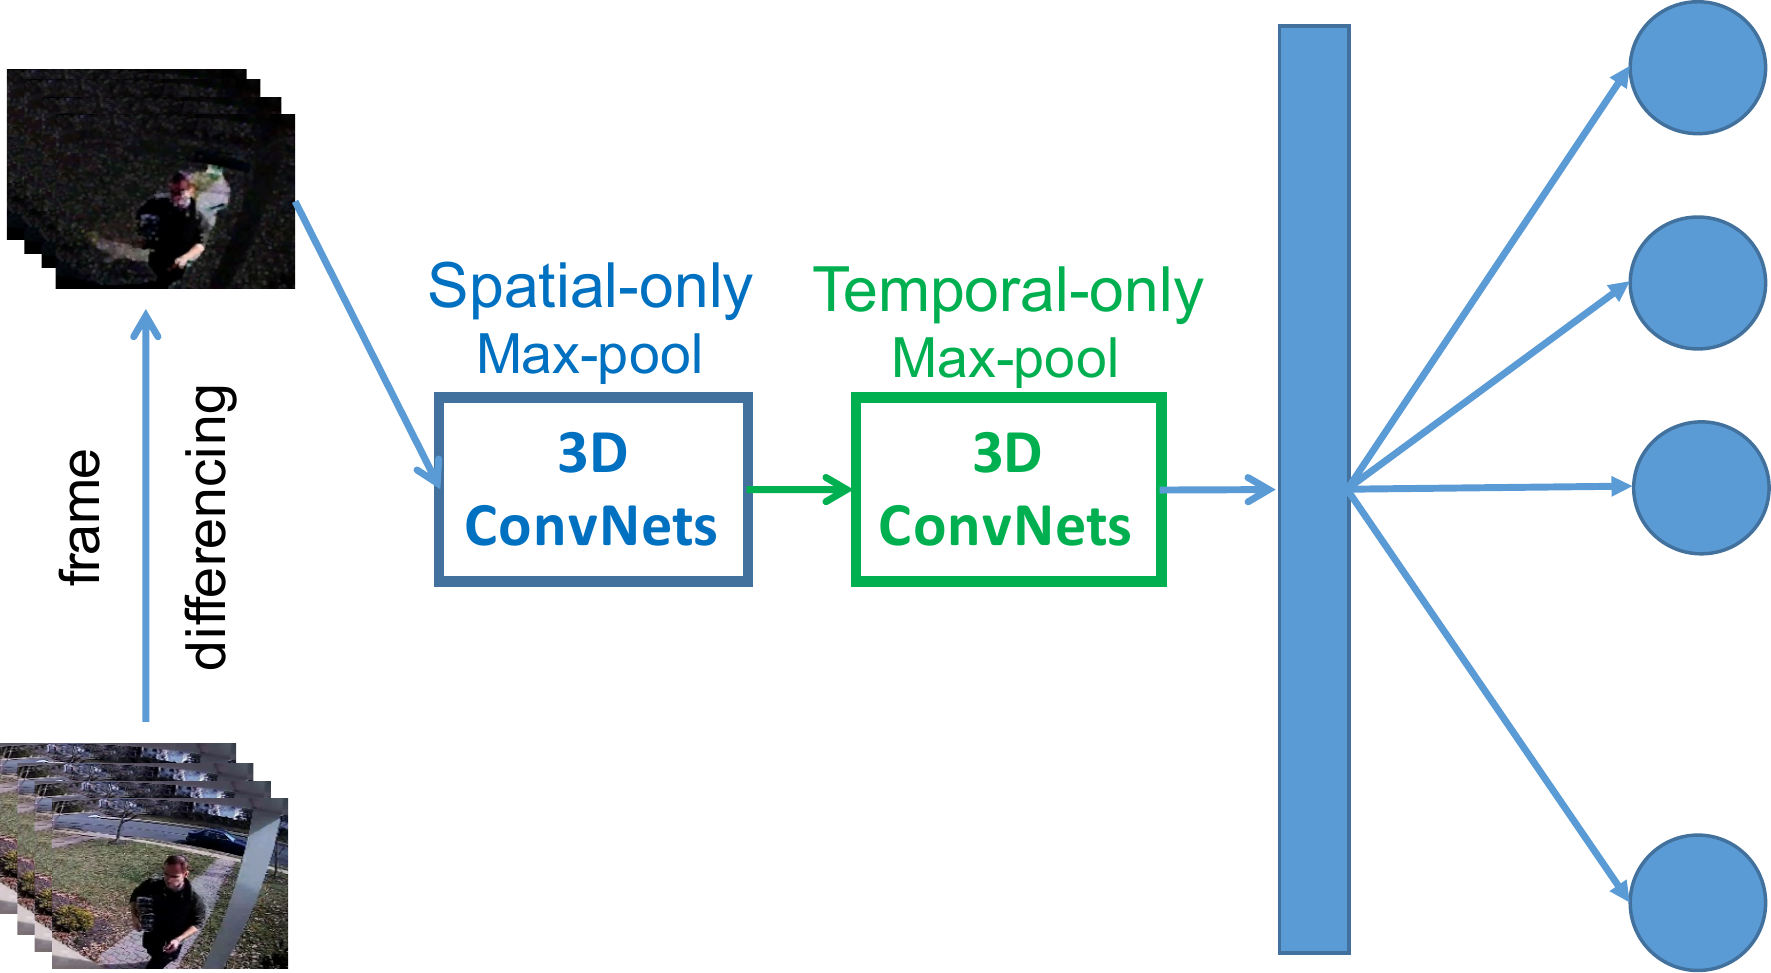}
%   \caption{Baseline model 1 (skip frame differencing) and 2 (with frame differencing}
% \label{fig:BL12}
% \end{figure}

% \begin{figure}[!t]
% \centering
%   \includegraphics[width=0.8\linewidth]{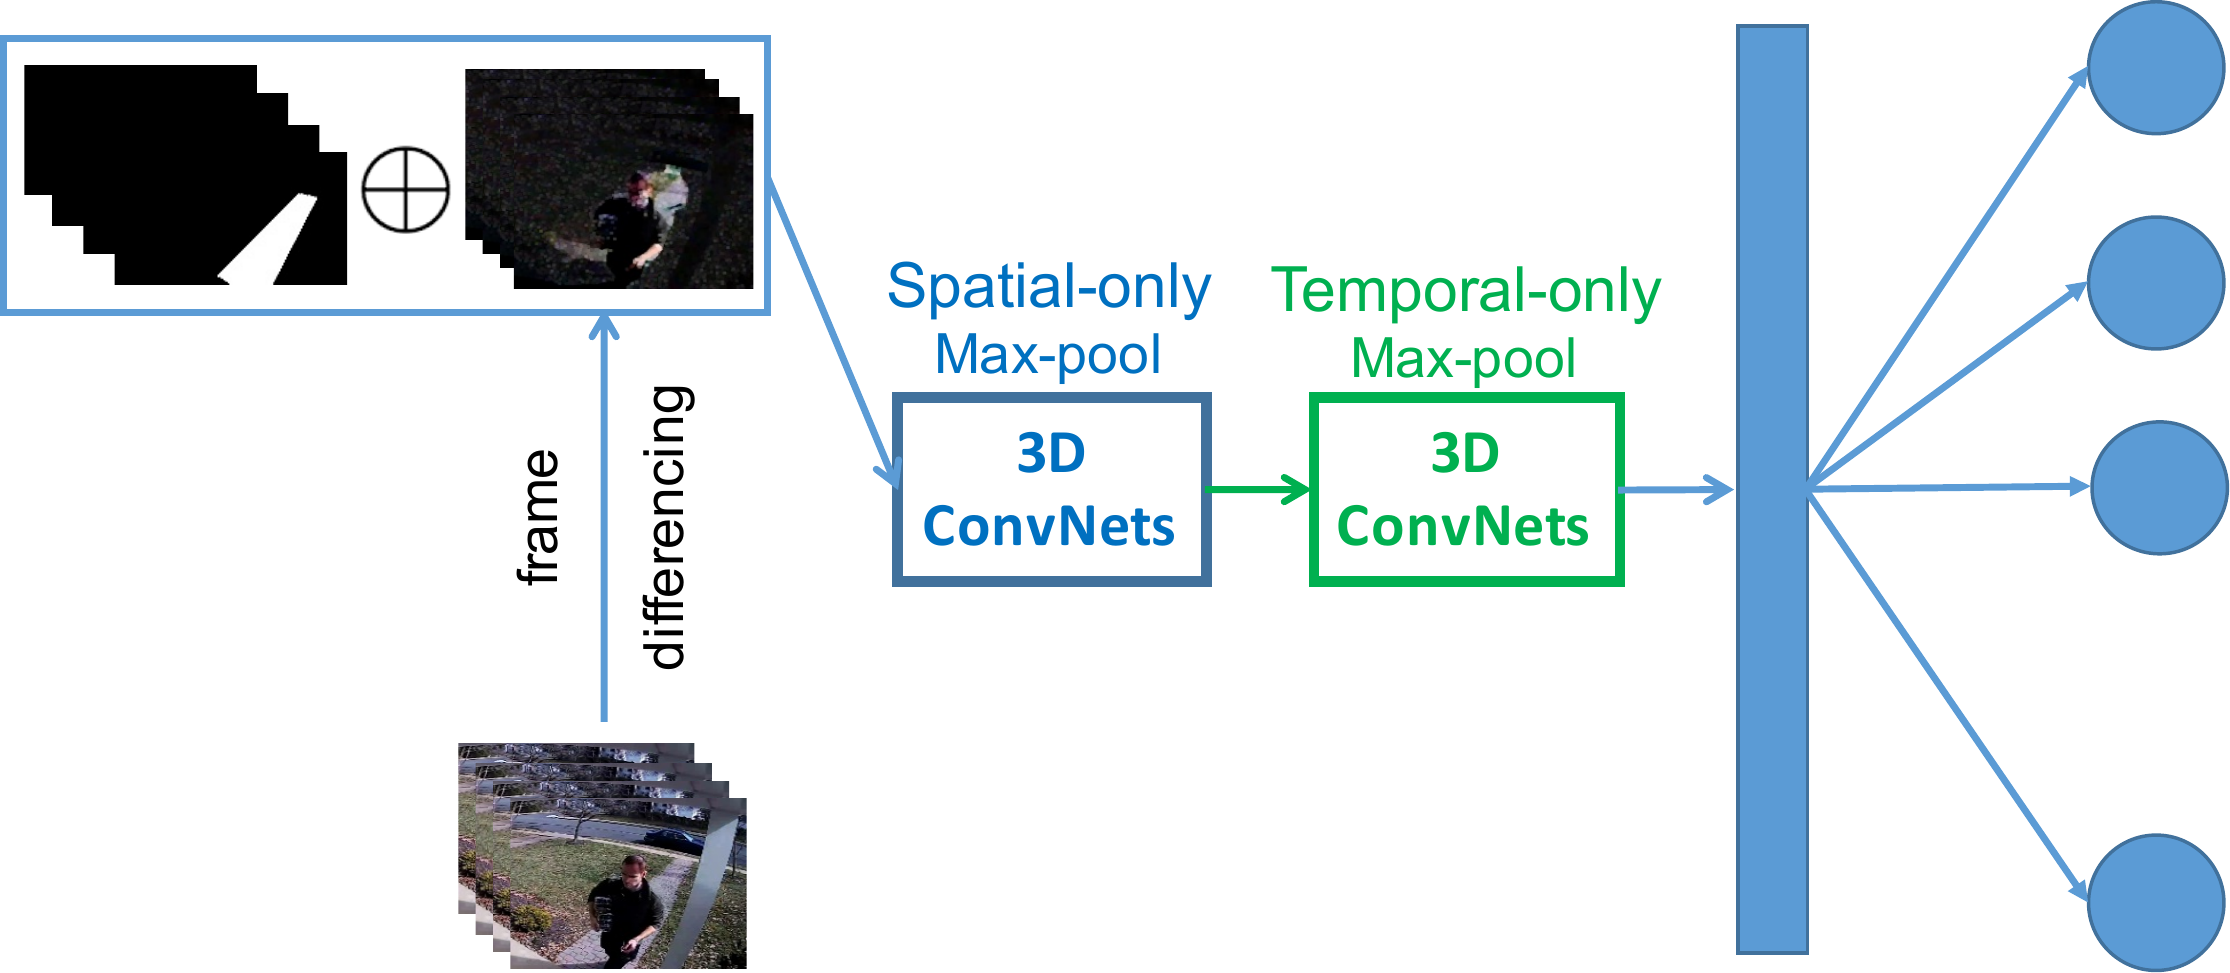}
%   \caption{Baseline 3. We directly stack the binary segmentation maps with the RGB channels of each frame, which leads to 9 channels in total to incorporate scene layout information. $\oplus$ denotes channel-wise concatenation.}
% \label{fig:BL3}
% \end{figure}

\begin{figure*}[!t]
\centering
  \subfigure[]{\label{fig:4}\includegraphics[width=0.45\linewidth]{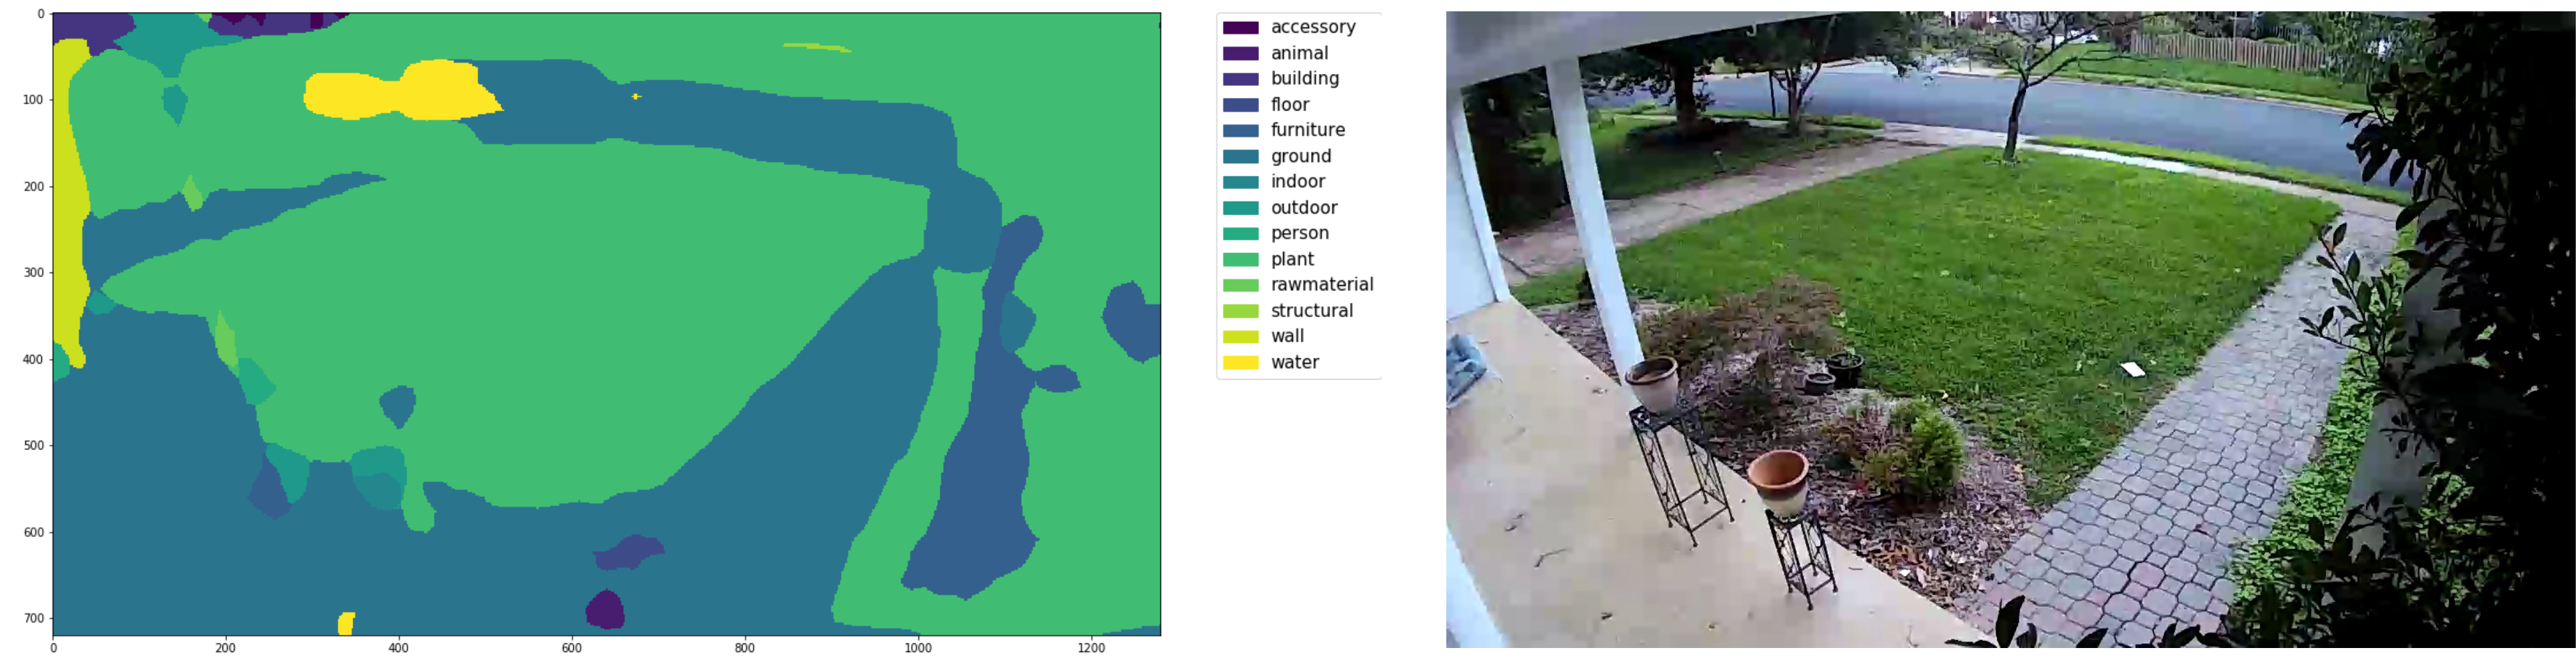}}
  \subfigure[]{\label{fig:1}\includegraphics[ width=0.45\linewidth]{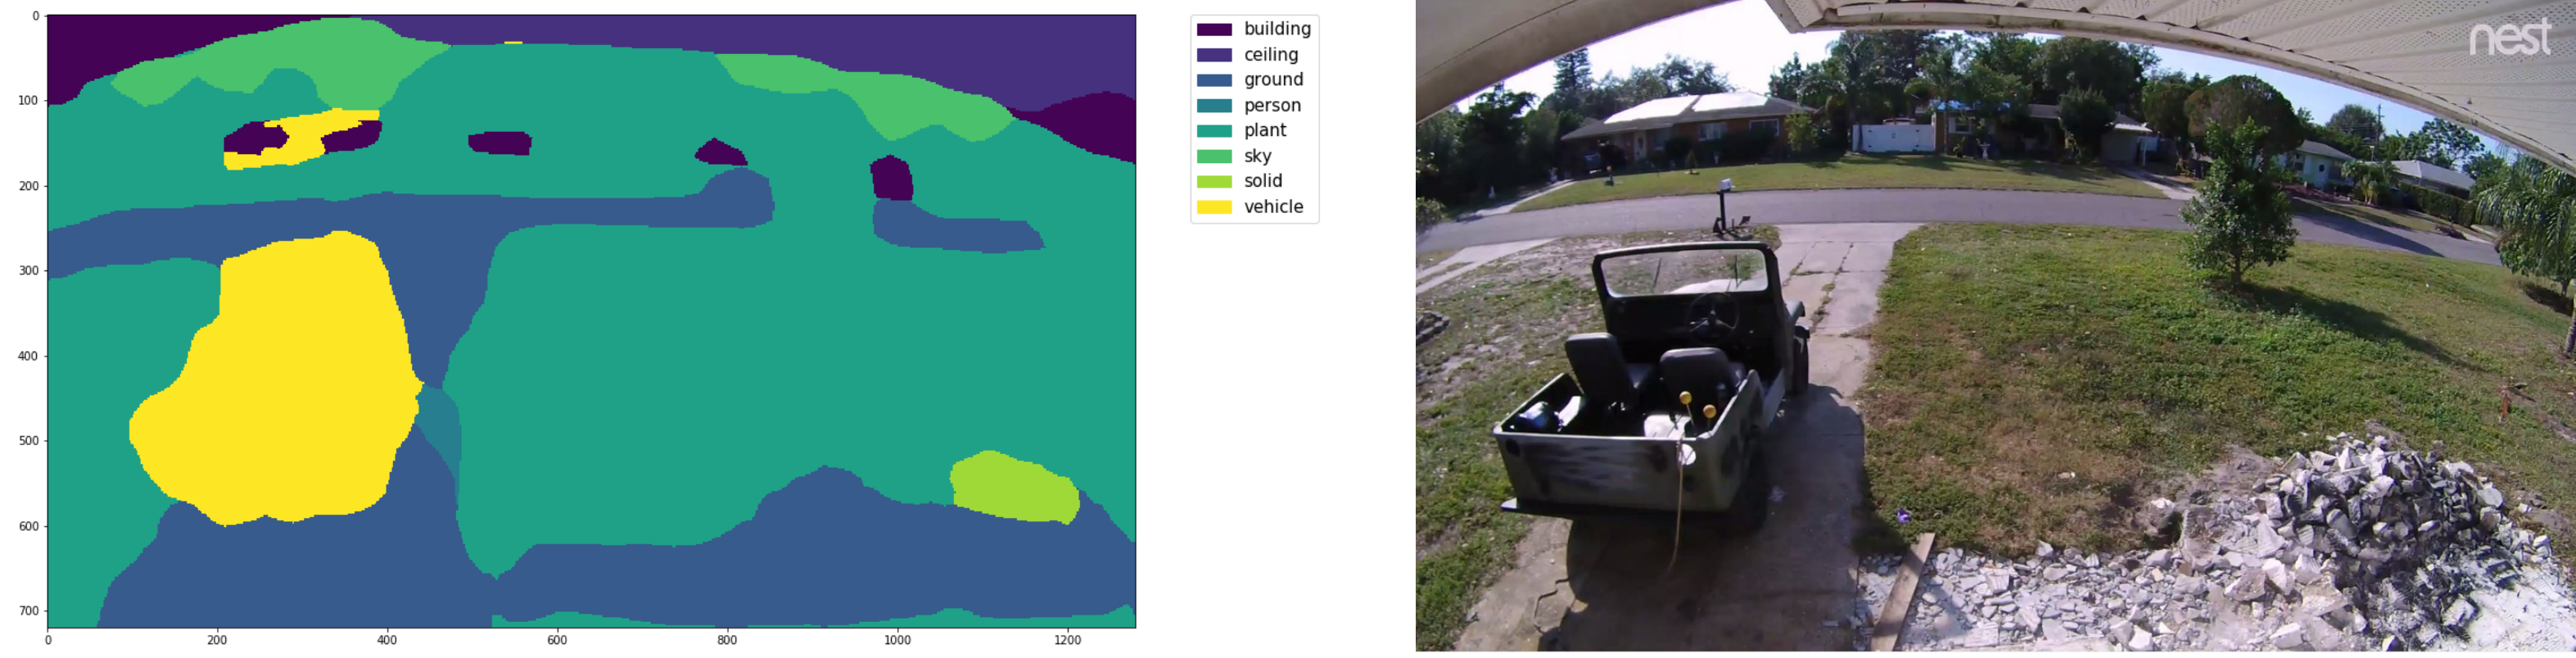}}
  
\subfigure[]{\label{fig:2}\includegraphics[ width=0.45\linewidth]{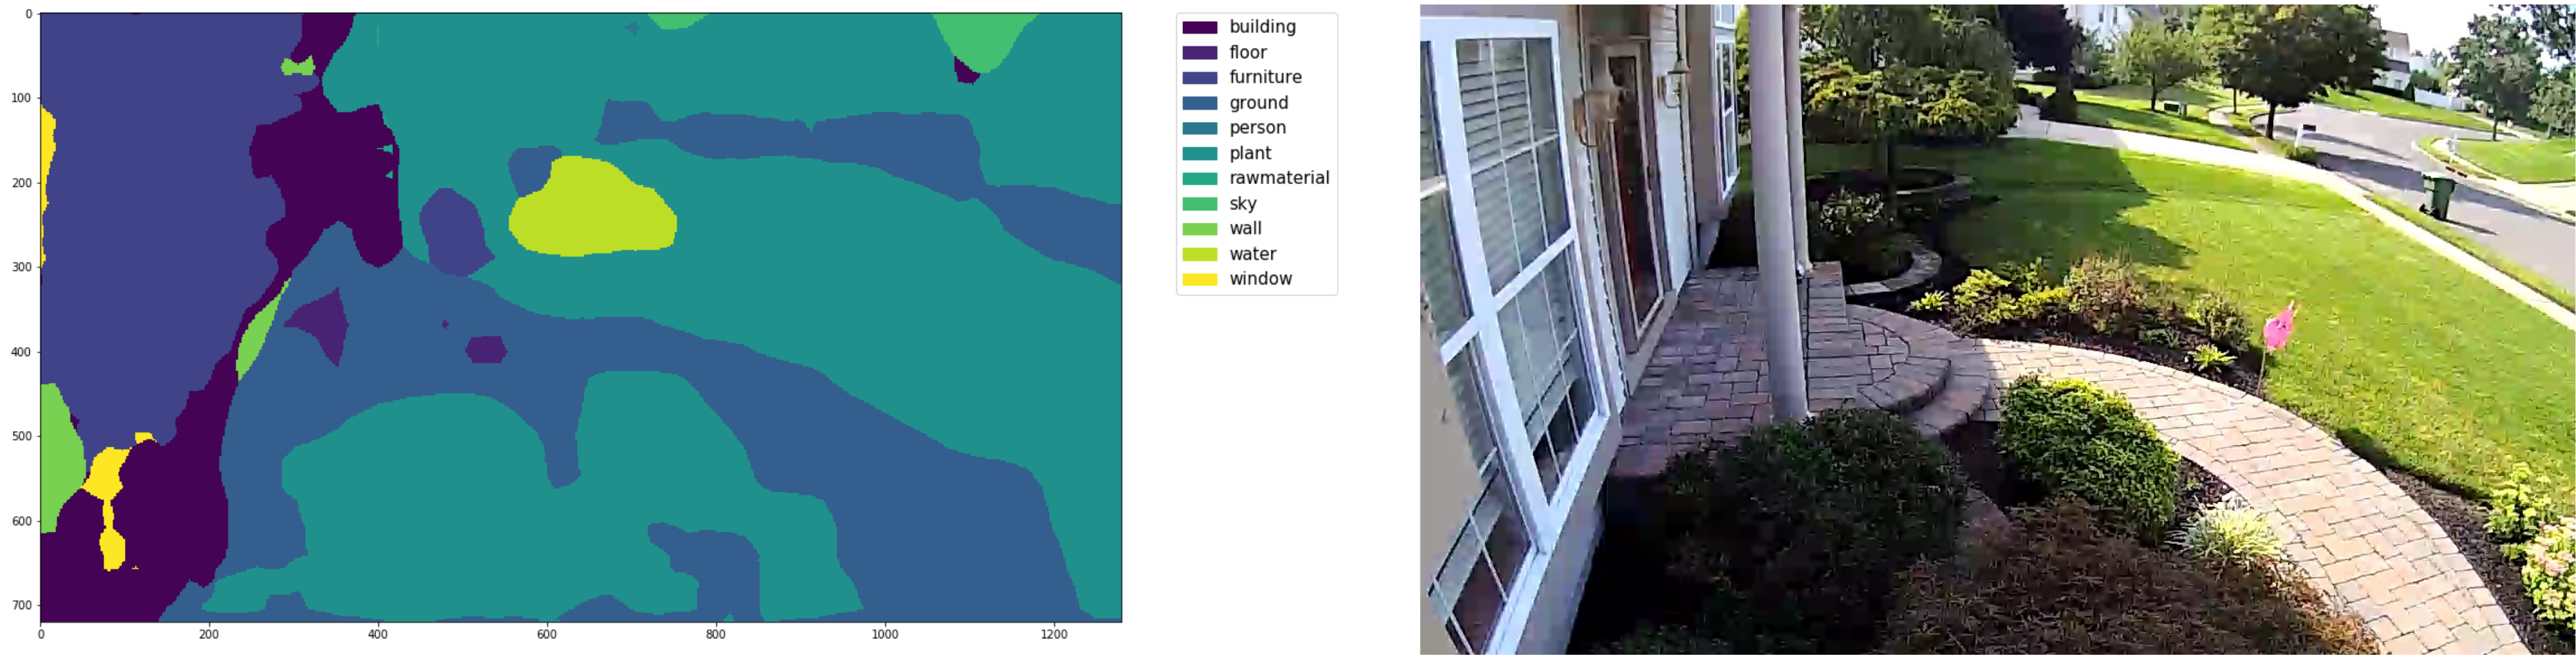}}
\subfigure[]{\label{fig:3}\includegraphics[ width=0.45\linewidth]{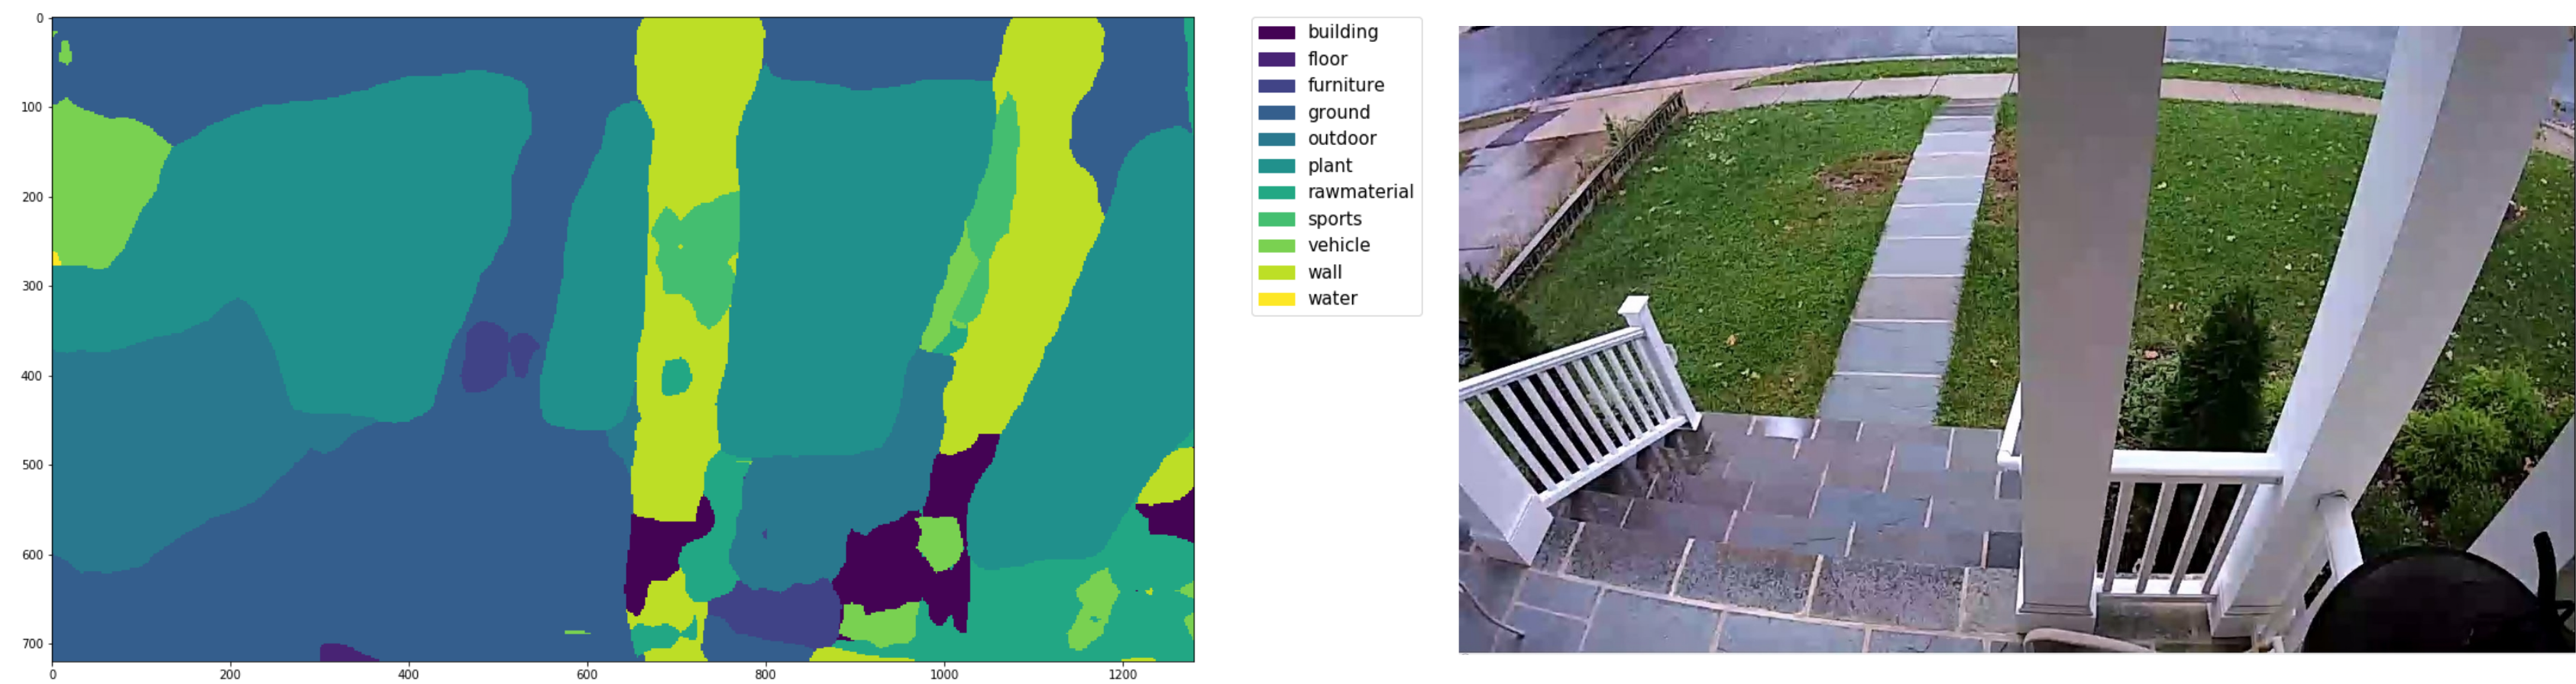}}
  \caption{Segmentation maps generated by Deeplab \cite{deeplab} V2 pre-trained on COCO-Stuff \cite{coco-stuff} dataset. Without enough training data, deep learning based method cannot precisely differentiate places with different functionalities (\eg walkway, driveway and street).}
\label{fig:deeplab}
\end{figure*}

\section{Automatically Generating Segmentation Maps}
In home surveillance scenario, we believe that it is reasonable to involve users to provide us with perfect segmentation maps of their own houses. However, to evaluate our proposed method's effectiveness with imperfect, automatically generated maps, we developed an algorithm using automatic semantic segmentation and historical statistics of the videos to generate place segmentation maps.

Due to the gap between appearance based segmentation (for most of the current semantic segmentation methods) and the functionality based segmentation (for our home surveillance scenario), directly applying the state of the art segmentation methods fails in our scenario. We applied Deeplab \cite{deeplab} V2 pre-trained on COCO-Stuff \cite{coco-stuff} dataset directly on our camera images and obtain poor results as shown in Fig.\ref{fig:deeplab}. 
From the figures we can see that the appearance-based segmentation methods assigns same labels to pixels with similar appearance but different functionalities. 
Without a large enough training dataset containing different scene layouts with functionality labels, it is difficult to apply deep learning based segmentation methods to generate the place segmentation maps. Thus instead, we propose an approach using low-level cues and historical statistics for automatic segmentation. We cluster pixels into super-pixels based on their appearance and spatial relations. Then, on these segments, we utilize normalized cut (NCut) \cite{Ncut}, which is an optimization based segmentation method, to further segment the images to multiple segments based on their appearance (Fig.\ref{fig:auto_all} (b)). 
Then, we apply a heuristic method that utilizes videos of the scenes to obtain heatmaps of some specific places (Fig.\ref{fig:auto_all} (c)), based on the fact that the object types and motion patterns on different functional places are different. For example, we can usually observe people/vehicles with different scales and walking in different ways at different functional places, from the view of a surveillance camera.
Based on the observations, we first apply object detection algorithm \cite{faster} and tracking algorithm \cite{sort} to detect and track moving person and vehicles in the videos, and then generate the heatmaps of porch, walkway, street, sidewalk and driveway in each scene based on the above heuristics.

% people walking along sidewalk and walkway. Considering the view of a surveillance camera, the scale of people on sidewalk is usually small due to the large distance from the sidewalk to the camera, while the one on walkway could be large; the changes for people's scale on sidewalk is also relatively small, while the changes could be large on walkway when people walk forward/away from home. Similar patterns can be observed on vehicles driving along street or driveway. To differentiate porch from walkway and sidewalk, we leverage the fact that people on porch are usually large and the changes of their scale is relatively small. 
% using Algorithm ~\ref{algo:heatmap}. 
% \begin{algorithm}[!t]
% \caption{}\label{algo:heatmap}
% \begin{algorithmic}[1]
% \State $\mathbf{Input: }  \text{Videos of a specific scene} \mathbf{V}, $
% \State $\text{, flattened importance of the $f^{th}$ output channel }$ \State $\mathbf{S}_{out}^f \in \mathbb{R}^ {1 \times( X \times X )}$
% \For {n in 1 \dots N}
% \For {f in 1 \dots F}
% \State $\mathbf{k}_{fn}  \gets |\mathbf{W}[:,:,n,f]|$
% \State $\text{Construct } \mathbf{BP}_{conv}^{fn}$ as \eqref{BP_conv} and \eqref{b_c}
% \State $\mathbf{S}_{in}^{fn} \gets \mathbf{S}_{out}^f \cdot
% \mathbf{BP}_{conv}^{fn}$
% \EndFor
% \State $\mathbf{S}_{in}^{n} \gets \sum_f \mathbf{S}_{in}^{fn}$
% \EndFor
% \State $\mathbf{S}_{in} \gets [\mathbf{S}_{in}^{1},\mathbf{S}_{in}^{2} \dots, \mathbf{S}_{in}^{N}]$
% \State \text{end}
% \end{algorithmic}
% \end{algorithm}

Given the results of NCut and the heatmaps, we label each segment with the majority place category of the heatmap. We label segments as lawn if their averaged color is close to one of the reference colors, \eg green, dark green, \etc 
The resulting annotation maps are shown in Fig.\ref{fig:auto_all}(d). When compared to the manually labeled ground truth, our automatically generated maps are reasonably good, especially for place categories such as walkway, porch, lawn and street. However, sometime our method may mistakenly label sidewalk or driveway as street. The NCut method cannot precisely separate sidewalk from street since sidewalk is usually a very narrow region in the camera view. Also, the appearance of sidewalk is very similar to street.
An interesting future direction of this work is to integrate the estimation of the semantic maps into the network architecture in an end-to-end trainable framework, which would require collecting more scenes for training.

\begin{figure*}[!t]
\centering
  \includegraphics[width=0.8\linewidth]{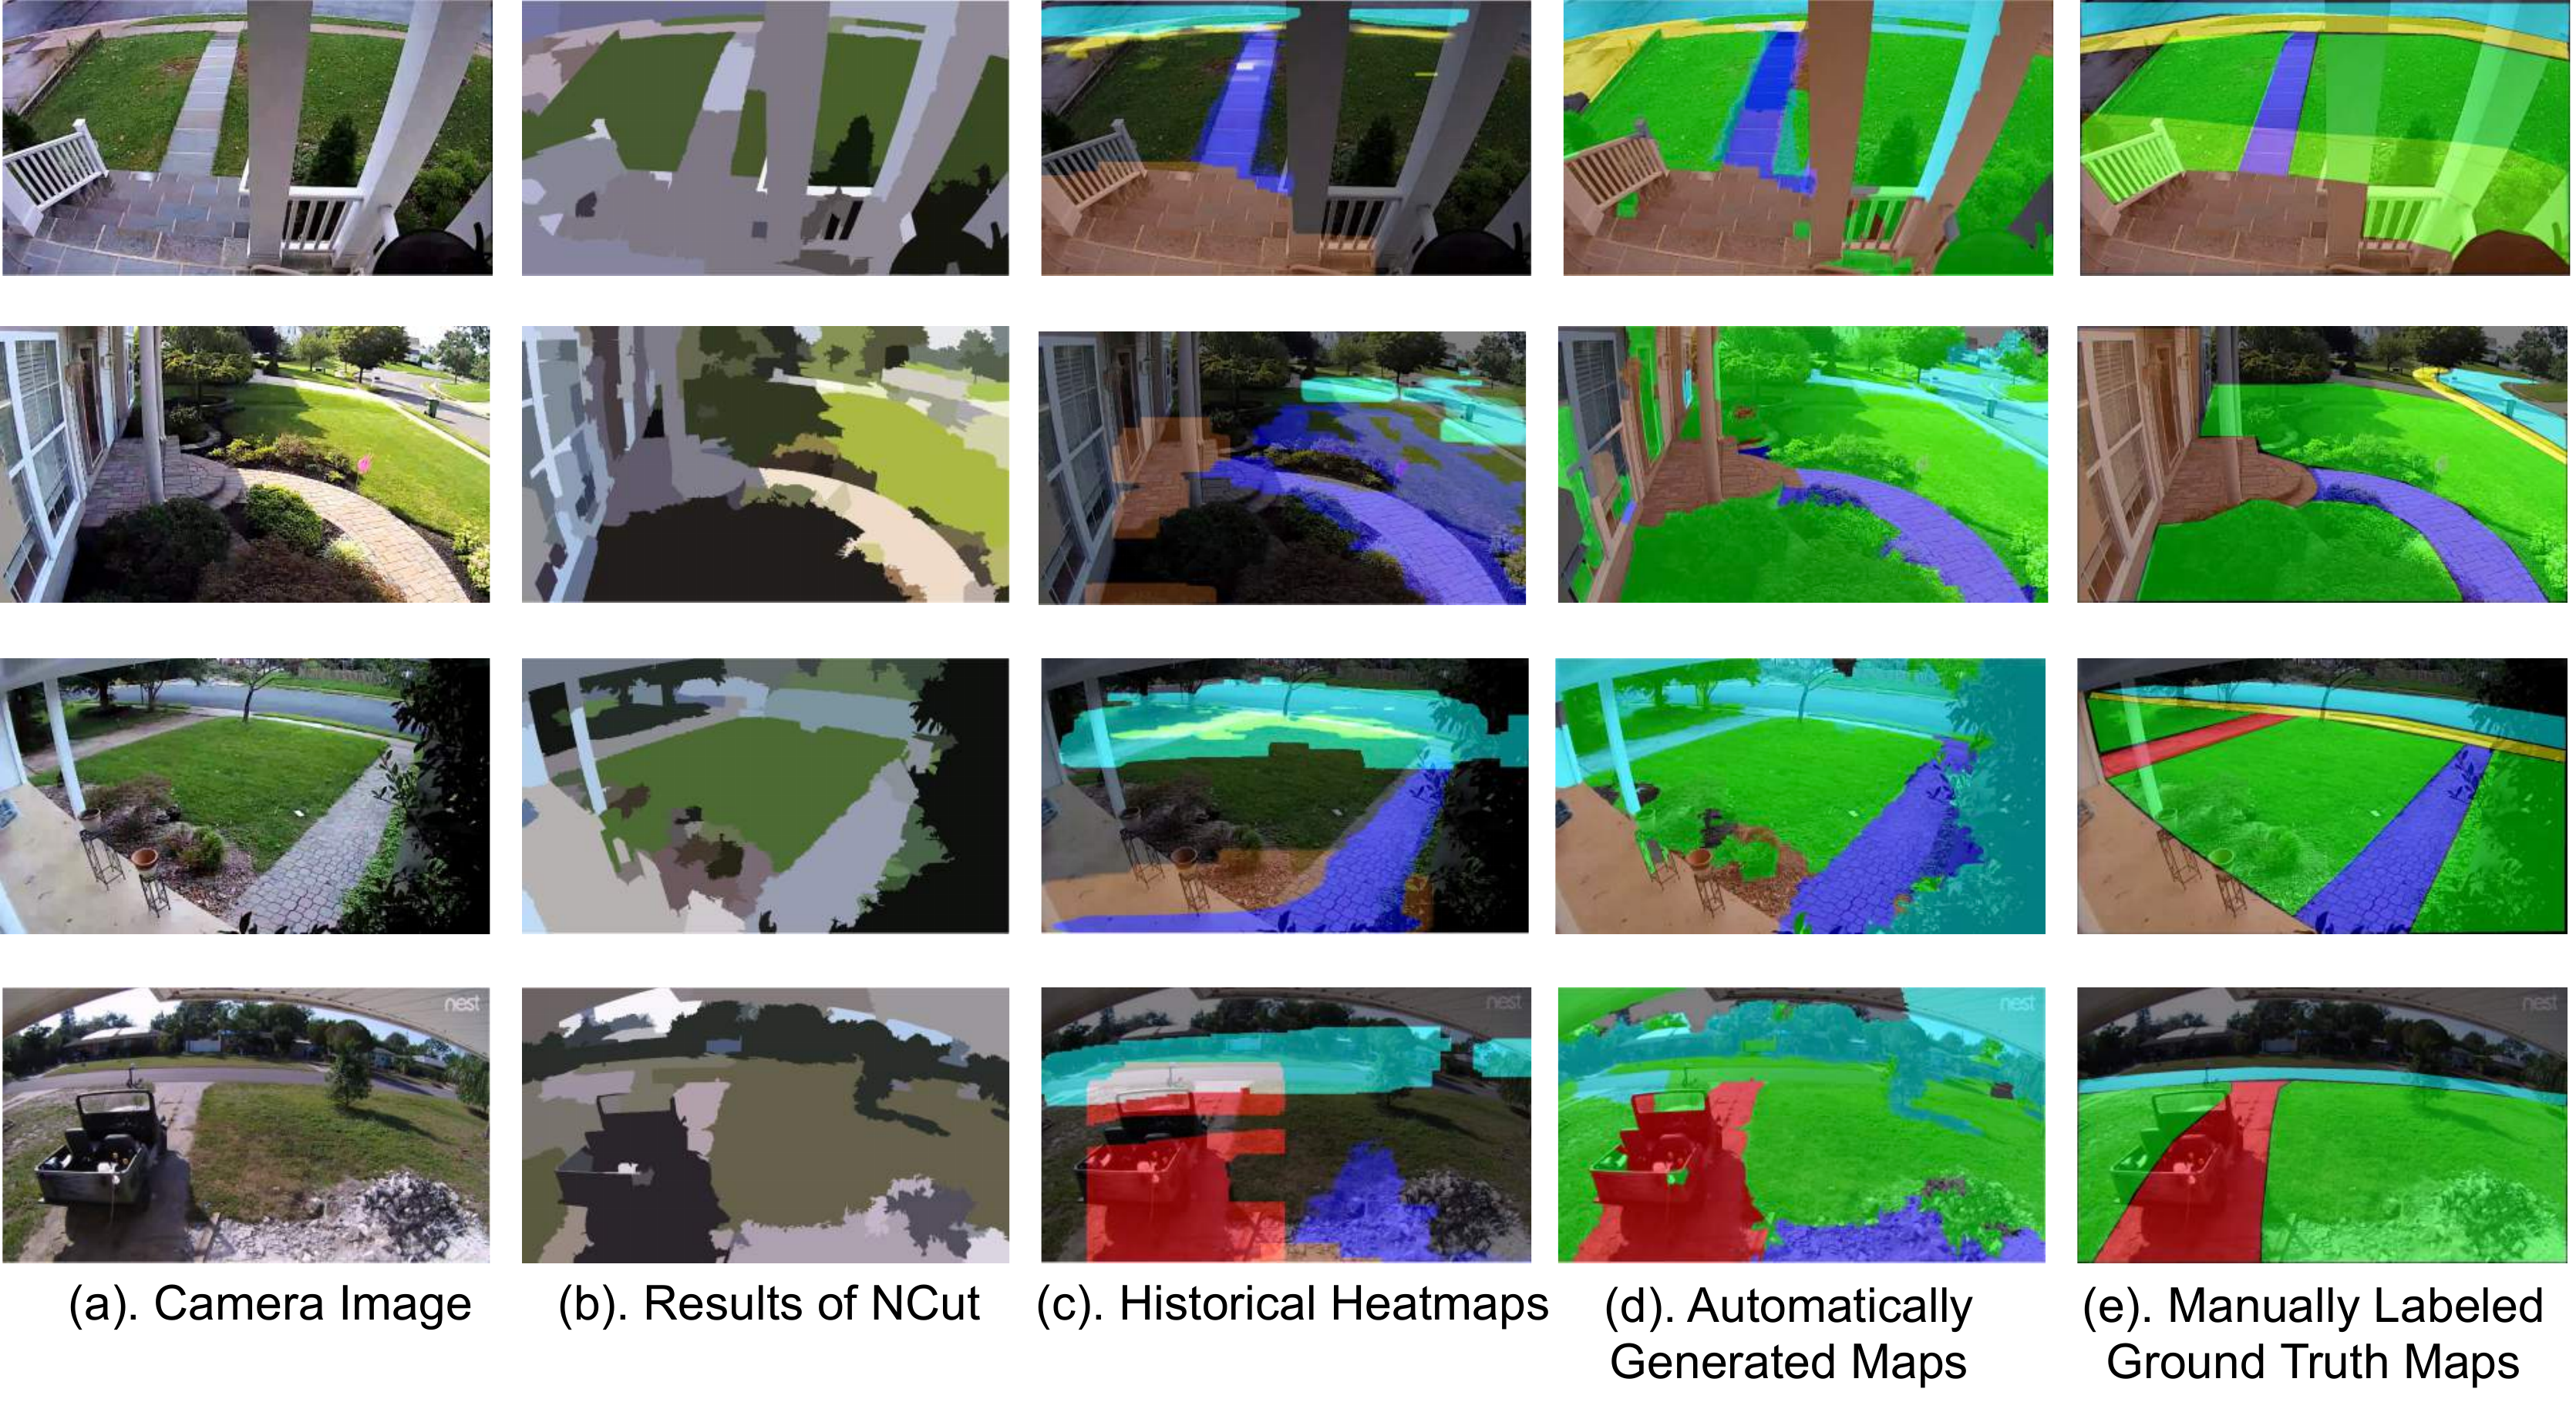}
  \caption{(a) shows the camera images. (b) shows the results of NCut. Each super pixel is represented using its color mean. (c) shows the heatmaps obtained from historical videos using our heuristic method. (d) shows the automatically generated maps. (e) shows the annotated maps. }
\label{fig:auto_all}
\end{figure*}
